# Supplementary material for: What are Asset Price Bubbles? A Survey on Definitions of Financial Bubbles
Source: arXiv:2502.10101 ancillary file (2025-02-14)
Supplement: Supplementary file 1 [file supplementary_material.pdf]

# Supplementary Material for the Paper “What are Asset Price Bubbles? A Survey on Definitions of Financial Bubbles”

Michael Heinrich Baumann<sup>1</sup> and Anja Janischewski<sup>2,\*</sup>

<sup>1</sup>Department of Mathematics, University of Bayreuth, Bayreuth, Germany, D-95447;

email: michael.baumann@uni-bayreuth.de

<sup>2</sup>Department of Economics and Business Administration,

Chemnitz University of Technology, Chemnitz, Germany, D-09126;

email: anja.janischewski@wiwi.tu-chemnitz.de

\*Corresponding author

February 14, 2025

Table 1: Categorization of the set of 122 papers in the systematic review along bubble definition categories. One paper out of the overall sample of 123 papers did not fit the topic of asset price bubbles [112].

| Definition category                           | Number of papers | Fractions | References                                                                                                                                                                |
|-----------------------------------------------|------------------|-----------|---------------------------------------------------------------------------------------------------------------------------------------------------------------------------|
| expected future cash flow                     | 41               | 0.34      | [7, 8, 9, 14, 15, 19, 20, 24, 25, 31, 32, 33, 36, 38, 40, 42, 47, 48, 53, 54, 58, 59, 64, 62, 65, 67, 70, 69, 74, 78, 87, 92, 97, 101, 102, 103, 105, 106, 111, 113, 120] |
| actual cash flows                             | 2                | 0.02      | [20, 104]                                                                                                                                                                 |
| utility                                       | 6                | 0.05      | [3, 5, 11, 12, 47, 75]                                                                                                                                                    |
| book value                                    | 6                | 0.05      | [7, 44, 68, 84, 85, 86]                                                                                                                                                   |
| market equilibrium                            | 12               | 0.10      | [2, 3, 9, 16, 23, 45, 49, 52, 56, 66, 110, 122]                                                                                                                           |
| heuristics                                    | 7                | 0.06      | [3, 7, 11, 22, 35, 63, 73]                                                                                                                                                |
| exogenously given                             | 27               | 0.22      | [1, 17, 29, 30, 36, 43, 46, 55, 57, 60, 61, 62, 68, 77, 79, 89, 90, 91, 93, 96, 98, 99, 100, 105, 109, 114, 119]                                                          |
| non-unique fundamental value                  | 3                | 0.02      | [28, 44, 119]                                                                                                                                                             |
| additional reference to price path properties | 19               | 0.16      | [9, 17, 26, 30, 36, 42, 43, 45, 46, 47, 57, 66, 67, 73, 75, 101, 109, 111, 120]                                                                                           |
| volatility                                    | 5                | 0.04      | [43, 47, 57, 71, 81]                                                                                                                                                      |
| boom                                          | 31               | 0.25      | [9, 13, 17, 21, 26, 30, 36, 37, 39, 42, 43, 45, 46, 51, 66, 67, 71, 72, 73, 75, 81, 83, 101, 107, 108, 109, 116, 117, 118, 121, 123]                                      |
| crash                                         | 11               | 0.09      | [9, 17, 21, 37, 46, 51, 71, 72, 73, 107, 109]                                                                                                                             |
| historical bubbles                            | 2                | 0.02      | [4, 95]                                                                                                                                                                   |
| other                                         | 3                | 0.02      | [26, 28, 80]                                                                                                                                                              |
| fits the topic but no definition present      | 12               | 0.10      | [6, 10, 18, 27, 34, 41, 50, 76, 82, 88, 94, 115]                                                                                                                          |

Table 2: Categorization of the set of 122 papers in the systematic review along research areas

| Research Area                               | Number of papers | References                                                                                                      |
|---------------------------------------------|------------------|-----------------------------------------------------------------------------------------------------------------|
| Heterogeneous Agents and Behavioral Finance | 8                | [1, 11, 13, 55, 60, 61, 110, 119]                                                                               |
| History and others (eg. Geography)          | 2                | [41, 82]                                                                                                        |
| Macro and General Economics                 | 12               | [10, 19, 28, 29, 57, 65, 76, 75, 77, 84, 85, 86]                                                                |
| Econophysics                                | 7                | [17, 21, 71, 72, 73, 95, 107]                                                                                   |
| Experimental Economics                      | 16               | [14, 15, 25, 31, 33, 36, 58, 59, 79, 87, 89, 91, 93, 98, 105, 106]                                              |
| (Crypto) Currency                           | 4                | [12, 43, 44, 56]                                                                                                |
| Real Estate and Housing                     | 23               | [4, 5, 7, 16, 20, 24, 26, 34, 35, 37, 45, 47, 48, 49, 63, 74, 81, 83, 94, 102, 103, 118, 120]                   |
| Commodities, Agricultur, and Energy         | 12               | [23, 39, 40, 52, 66, 78, 88, 96, 101, 111, 122, 123]                                                            |
| Mathematical Finance                        | 4                | [67, 68, 70, 69]                                                                                                |
| Policy and Politics                         | 5                | [18, 22, 27, 100, 115]                                                                                          |
| Finance and Banking                         | 27               | [2, 6, 8, 9, 30, 32, 38, 42, 46, 50, 51, 53, 54, 64, 62, 80, 90, 92, 97, 99, 104, 108, 109, 113, 116, 117, 121] |
| Trade                                       | 2                | [3, 114]                                                                                                        |

Table 3: Categorization of the set of 122 papers along type of analysis (theoretical or applied)

| Paper type (theoretical or applied) | Number of papers | References                                                                                                                                                                                                                                                                       |
|-------------------------------------|------------------|----------------------------------------------------------------------------------------------------------------------------------------------------------------------------------------------------------------------------------------------------------------------------------|
| theoretical paper                   | 34               | [1, 2, 5, 9, 13, 18, 23, 27, 28, 29, 30, 37, 38, 42, 46, 53, 55, 57, 60, 61, 62, 68, 70, 69, 76, 77, 84, 85, 92, 95, 97, 110, 114, 119]                                                                                                                                          |
| applied paper                       | 66               | [3, 4, 6, 7, 10, 12, 14, 15, 16, 19, 20, 22, 24, 25, 26, 31, 32, 33, 35, 39, 40, 41, 43, 44, 45, 48, 50, 51, 52, 54, 56, 58, 59, 64, 63, 66, 71, 74, 75, 79, 80, 81, 82, 83, 87, 88, 89, 90, 91, 93, 94, 96, 98, 99, 101, 102, 103, 105, 106, 111, 115, 118, 120, 121, 122, 123] |
| both, theory and applied            | 22               | [8, 11, 17, 21, 30, 36, 47, 49, 65, 67, 72, 73, 78, 86, 100, 104, 107, 108, 109, 113, 116, 117]                                                                                                                                                                                  |

Table 4: Categorization along type of definition (formal or with words; if formal: discrete or continuous time formula) for the papers in which a definition is present. (Multiple mentions possible, only papers with definition considered, i.e. 110 papers).

| Definition type: formal or with words | Number of papers | References                                                                                                                                                                                                                                                                                     |
|---------------------------------------|------------------|------------------------------------------------------------------------------------------------------------------------------------------------------------------------------------------------------------------------------------------------------------------------------------------------|
| Formal, discrete                      | 69               | [2, 3, 5, 7, 8, 9, 11, 12, 14, 15, 16, 19, 20, 24, 25, 28, 32, 33, 36, 38, 39, 40, 44, 47, 48, 49, 53, 54, 55, 56, 57, 58, 59, 60, 61, 64, 62, 63, 65, 71, 73, 74, 77, 78, 80, 81, 86, 87, 90, 92, 93, 97, 98, 100, 101, 102, 103, 105, 106, 110, 111, 113, 114, 116, 118, 120, 121, 122, 123] |
| Formal, continuous                    | 16               | [17, 21, 30, 42, 43, 46, 67, 68, 70, 69, 72, 84, 85, 109, 117, 119]                                                                                                                                                                                                                            |
| with words                            | 37               | [1, 3, 4, 7, 9, 13, 22, 23, 26, 28, 29, 31, 35, 37, 42, 45, 46, 51, 52, 56, 57, 61, 66, 73, 75, 77, 79, 81, 83, 89, 91, 95, 96, 99, 104, 107, 108]                                                                                                                                             |

## References

- [1] D. Abreu and M. Brunnermeir. Bubbles and crashes. *Econometrica*, 71(1):173–204, 2003. cited By 453.
- [2] V. Acharya and H. Naqvi. The seeds of a crisis: A theory of bank liquidity and risk taking over the business cycle. *Journal of Financial Economics*, 106(2):349–366, 2012. cited By 202.
- [3] R. Adland, R. Adland, H. Jia, and S. Strandenes. Asset bubbles in shipping? an analysis of recent history in the drybulk market. *Maritime Economics and Logistics*, 8(3):223–233, 2006. cited By 20.
- [4] O. Akin, J. Montalvo, J. García Villar, J.-L. Peydró, and J. Raya. The real estate and credit bubble: evidence from spain. *SERIEs*, 5(2-3):223–243, 2014. cited By 39.
- [5] F. Allen and E. Carletti. Systemic risk from real estate and macro-prudential regulation. *International Journal of Banking, Accounting and Finance*, 5(1-2):28–48, 2013. cited By 25.
- [6] F. Allen and E. Carletti. What is systemic risk? *Journal of Money, Credit and Banking*, 45(SUPPL 1):121–127, 2013. cited By 37.
- [7] B. Ambrose, P. Eichholtz, and T. Lindenthal. House prices and fundamentals: 355 years of evidence. *Journal of Money, Credit and Banking*, 45(2-3):477–491, 2013. cited By 64.
- [8] K. Anderson, C. Brooks, and A. Katsaris. Speculative bubbles in the s&p 500: Was the tech bubble confined to the tech sector? *Journal of Empirical Finance*, 17(3):345–361, 2010. cited By 37.
- [9] N. Barberis, R. Greenwood, L. Jin, and A. Shleifer. Extrapolation and bubbles. *Journal of Financial Economics*, 129(2):203–227, 2018. cited By 60.
- [10] R. Barrell and E. Davis. The evolution of the financial crisis of 2007-8. *National Institute Economic Review*, 206(1):5–14, 2008. cited By 32.
- [11] D. Baur and K. Glover. Heterogeneous expectations in the gold market: Specification and estimation. *Journal of Economic Dynamics and Control*, 40:116–133, 2014. cited By 22.
- [12] J. Białkowski, M. Bohl, P. Stephan, and T. Wisniewski. The gold price in times of crisis. *International Review of Financial Analysis*, 41:329–339, 2015. cited By 54.
- [13] A. Biondo, A. Pluchino, A. Rapisarda, and D. Helbing. Reducing financial avalanches by random investments. *Physical Review E - Statistical, Nonlinear, and Soft Matter Physics*, 88(6), 2013. cited By 30.
- [14] C. Bosch-Rosa, T. Meissner, and A. Bosch-Domènech. Cognitive bubbles. *Experimental Economics*, 21(1):132–153, 2018. cited By 27.
- [15] A. Bostian and C. Holt. Price bubbles with discounting: A web-based classroom experiment. *Journal of Economic Education*, 40(1):27–37, 2009. cited By 20.
- [16] S. Bourassa, P. Hendershott, and J. Murphy. Further evidence on the existence of housing market bubbles. *Journal of Property Research*, 18(1):1–19, 2001. cited By 37.
- [17] D. Brée and N. Joseph. Testing for financial crashes using the log periodic power law model. *International Review of Financial Analysis*, 30:287–297, 2013. cited By 20.
- [18] S. Breslin. China and the crisis: Global power, domestic caution and local initiative. *Contemporary Politics*, 17(2):185–200, 2011. cited By 25.

- [19] C. Brooks and A. Katsaris. Rational speculative bubbles: An empirical investigation of the london stock exchange. *Bulletin of Economic Research*, 55(4):319–346, 2003. cited By 48.
- [20] C. Brooks, A. Katsaris, T. McGough, and S. Tsolacos. Testing for bubbles in indirect property price cycles. *Journal of Property Research*, 18(4):341–356, 2001. cited By 21.
- [21] D. Cajueiro, B. Tabak, and F. Werneck. Can we predict crashes? the case of the brazilian stock market. *Physica A: Statistical Mechanics and its Applications*, 388(8):1603–1609, 2009. cited By 18.
- [22] M. Campello and J. Graham. Do stock prices influence corporate decisions? evidence from the technology bubble. *Journal of Financial Economics*, 107(1):89–110, 2013. cited By 63.
- [23] C. Carter, G. Rausser, and A. Smith. Commodity booms and busts. *Annual Review of Resource Economics*, 3:87–118, 2011. cited By 75.
- [24] H. Chan, S. Lee, and K. Woo. Detecting rational bubbles in the residential housing markets of hong kong. *Economic Modelling*, 18(1):61–73, 2001. cited By 47.
- [25] S. Cheung and S. Palan. Two heads are less bubbly than one: Team decision-making in an experimental asset market. *Experimental Economics*, 15(3):373–397, 2012. cited By 21.
- [26] G. Clark, R. Durán-Fernández, and K. Strauss. Being in the market’: The uk house-price bubble and the intended structure of individual pension investment portfolios. *Journal of Economic Geography*, 10(3):331–359, 2010. cited By 16.
- [27] R. Congleton. On the political economy of the financial crisis and bailout of 2008-2009. *Public Choice*, 140(3-4):287–317, 2009. cited By 48.
- [28] J. Conlon. Simple finite horizon bubbles robust to higher order knowledge. *Econometrica*, 72(3):927–936, 2004. cited By 28.
- [29] G. Connor, T. Flavin, and B. O’Kelly. The u.s. and irish credit crises: Their distinctive differences and common features. *Journal of International Money and Finance*, 31(1):60–79, 2012. cited By 20.
- [30] F. Corsi and D. Sornette. Follow the money: The monetary roots of bubbles and crashes. *International Review of Financial Analysis*, 32:47–59, 2014. cited By 18.
- [31] C. Cueva and A. Rustichini. Is financial instability male-driven? gender and cognitive skills in experimental asset markets. *Journal of Economic Behavior and Organization*, 119:330–344, 2015. cited By 26.
- [32] J. Cuñado, L. Gil-Alana, and F. de Gracia. A test for rational bubbles in the nasdaq stock index: A fractionally integrated approach. *Journal of Banking and Finance*, 29(10):2633–2654, 2005. cited By 68.
- [33] C. Deck, D. Porter, and V. Smith. Double bubbles in assets markets with multiple generations. *Journal of Behavioral Finance*, 15(2):79–88, 2014. cited By 19.
- [34] W. Diewert, A. Nakamura, and L. Nakamura. The housing bubble and a new approach to accounting for housing in a cpi. *Journal of Housing Economics*, 18(3):156–171, 2009. cited By 25.
- [35] C. Dreger and Y. Zhang. Is there a bubble in the chinese housing market? *Urban Policy and Research*, 31(1):27–39, 2013. cited By 59.

- [36] J. Duffy and M. Ünver. Asset price bubbles and crashes with near-zero-intelligence traders. *Economic Theory*, 27(3):537–563, 2006. cited By 33.
- [37] M. Ebrahim. Can an islamic model of housing finance cooperative elevate the economic status of the underprivileged? *Journal of Economic Behavior and Organization*, 72(3):864–883, 2009. cited By 21.
- [38] T. Engsted and B. Nielsen. Testing for rational bubbles in a coexplosive vector autoregression. *Econometrics Journal*, 15(2):226–254, 2012. cited By 22.
- [39] R. Esposti and G. Listorti. Agricultural price transmission across space and commodities during price bubbles. *Agricultural Economics (United Kingdom)*, 44(1):125–139, 2013. cited By 44.
- [40] A. Featherstone and T. Baker. An examination of farm sector real asset dynamics: 1910–85. *American Journal of Agricultural Economics*, 69(3):532–546, 1987. cited By 73.
- [41] R. Frehen, W. Goetzmann, and K. Geert Rouwenhorst. New evidence on the first financial bubble. *Journal of Financial Economics*, 108(3):585–607, 2013. cited By 21.
- [42] D. Friedman and R. Abraham. Bubbles and crashes: Gradient dynamics in financial markets. *Journal of Economic Dynamics and Control*, 33(4):922–937, 2009. cited By 31.
- [43] J. Fry and E.-T. Cheah. Negative bubbles and shocks in cryptocurrency markets. *International Review of Financial Analysis*, 47:343–352, 2016. cited By 187.
- [44] D. Garcia, C. Tessone, P. Mavrodiev, and N. Perony. The digital traces of bubbles: Feedback cycles between socio-economic signals in the bitcoin economy. *Journal of the Royal Society Interface*, 11(99), 2014. cited By 198.
- [45] P. Gelain, K. Lansing, and G. Natvik. Explaining the boom–bust cycle in the u.s. housing market: A reverse-engineering approach. *Journal of Money, Credit and Banking*, 50(8):1751–1783, 2018. cited By 16.
- [46] S. Girdzijauskas and D. Štreimikiene. Application of logistic models for stock market bubbles analysis. *Journal of Business Economics and Management*, 10(1):45–51, 2009. cited By 16.
- [47] E. Glaeser and C. Nathanson. Housing bubbles. *Handbook of Regional and Urban Economics*, 5:701–751, 2015. cited By 24.
- [48] J. Gomez-Gonzalez, J. Gamboa-Arbeláez, J. Hirs-Garzón, and A. Pinchao-Rosero. When bubble meets bubble: Contagion in oecd countries. *Journal of Real Estate Finance and Economics*, 56(4):546–566, 2018. cited By 17.
- [49] A. Goodman and T. Thibodeau. Where are the speculative bubbles in us housing markets? *Journal of Housing Economics*, 17(2):117–137, 2008. cited By 100.
- [50] R. Greenwood and S. Nagel. Inexperienced investors and bubbles. *Journal of Financial Economics*, 93(2):239–258, 2009. cited By 127.
- [51] R. Greenwood, A. Shleifer, and Y. You. Bubbles for fama. *Journal of Financial Economics*, 131(1):20–43, 2019. cited By 21.
- [52] M. Gronwald. Explosive oil prices. *Energy Economics*, 60:1–5, 2016. cited By 25.
- [53] R. Gürkaynak. Econometric tests of asset price bubbles: Taking stock. *Journal of Economic Surveys*, 22(1):166–186, 2008. cited By 182.

- [54] L. Gutierrez. Bootstrapping asset price bubbles. *Economic Modelling*, 28(6):2488–2493, 2011. cited By 16.
- [55] G. HARRAS and D. Sornette. How to grow a bubble: A model of myopic adapting agents. *Journal of Economic Behavior and Organization*, 80(1):137–152, 2011. cited By 50.
- [56] A. Hayes. Bitcoin price and its marginal cost of production: support for a fundamental value. *Applied Economics Letters*, 26(7):554–560, 2019. cited By 25.
- [57] T. Hirano and N. Yanagawa. Asset bubbles, endogenous growth, and financial frictions. *Review of Economic Studies*, 84(1):406–443, 2017. cited By 34.
- [58] S. Hirota and S. Sunder. Price bubbles sans dividend anchors: Evidence from laboratory stock markets. *Journal of Economic Dynamics and Control*, 31(6):1875–1909, 2007. cited By 39.
- [59] C. Holt, M. Porzio, and M. Song. Price bubbles, gender, and expectations in experimental asset markets. *European Economic Review*, 100:72–94, 2017. cited By 21.
- [60] U. Horst. Financial price fluctuations in a stock market model with many interacting agents. *Economic Theory*, 25(4):917–932, 2005. cited By 31.
- [61] C. Hott. Herding behavior in asset markets. *Journal of Financial Stability*, 5(1):35–56, 2009. cited By 32.
- [62] K. Huang and J. Werner. Asset price bubbles in arrow-debreu and sequential equilibrium. *Economic Theory*, 15(2):253–278, 2000. cited By 27.
- [63] E. Hui and S. Yue. Housing price bubbles in hong kong, beijing and shanghai: A comparative study. *Journal of Real Estate Finance and Economics*, 33(4):299–327, 2006. cited By 169.
- [64] E.-M. Hui, I. Ng, and O.-F. Lau. Speculative bubbles in mass and luxury properties: An investigation of the hong kong residential market. *Construction Management and Economics*, 29(8):781–793, 2011. cited By 18.
- [65] J. In’t Veld, R. Raciborski, M. Ratto, and W. Roeger. The recent boom-bust cycle: The relative contribution of capital flows, credit supply and asset bubbles. *European Economic Review*, 55(3):386–406, 2011. cited By 30.
- [66] S. Irwin and D. Sanders. Index funds, financialization, and commodity futures markets. *Applied Economic Perspectives and Policy*, 33(1):1–31, 2011. cited By 211.
- [67] R. Jarrow, Y. Kchia, and P. Protter. How to detect an asset bubble. *SIAM Journal on Financial Mathematics*, 2(1):839–865, 2011. cited By 43.
- [68] R. Jarrow, P. Protter, and A. Roch. A liquidity-based model for asset price bubbles. *Quantitative Finance*, 12(9):1339–1349, 2012. cited By 16.
- [69] R. Jarrow, P. Protter, and K. Shimbo. Asset price bubbles in complete markets. *Applied and Numerical Harmonic Analysis*, (9780817645441):97–121, 2007. cited By 45.
- [70] R. Jarrow, P. Protter, and K. Shimbo. Asset price bubbles in incomplete markets. *Mathematical Finance*, 20(2):145–185, 2010. cited By 84.
- [71] Z.-Q. Jiang, W.-X. Zhou, D. Sornette, R. Woodard, K. Bastiaensen, and P. Cauwels. Bubble diagnosis and prediction of the 2005-2007 and 2008-2009 chinese stock market bubbles. *Journal of Economic Behavior and Organization*, 74(3):149–162, 2010. cited By 128.

- [72] A. Johansen. Characterization of large price variations in financial markets. *Physica A: Statistical Mechanics and its Applications*, 324(1-2):157–166, 2003. cited By 42.
- [73] T. Kaizoji. Speculative bubbles and crashes in stock markets: An interacting-agent model of speculative activity. *Physica A: Statistical Mechanics and its Applications*, 287(3-4):493–506, 2000. cited By 98.
- [74] W. Koh, R. Mariano, A. Pavlov, S. Phang, A. Tan, and S. Wachter. Bank lending and real estate in asia: Market optimism and asset bubbles. *Journal of Asian Economics*, 15(6):1103–1118, 2005. cited By 18.
- [75] D. Kotz. Contradictions of economic growth in the neoliberal era: Accumulation and crisis in the contemporary u.s. economy. *Review of Radical Political Economics*, 40(2):174–188, 2008. cited By 36.
- [76] D. Kotz. The financial and economic crisis of 2008: A systemic crisis of neoliberal capitalism. *Review of Radical Political Economics*, 41(3):305–317, 2009. cited By 181.
- [77] T. Kunieda and A. Shibata. Asset bubbles, economic growth, and a self-fulfilling financial crisis. *Journal of Monetary Economics*, 82:70–84, 2016. cited By 16.
- [78] M. Lammerding, P. Stephan, M. Trede, and B. Wilfling. Speculative bubbles in recent oil price dynamics: Evidence from a bayesian markov-switching state-space approach. *Energy Economics*, 36:491–502, 2013. cited By 61.
- [79] V. Lei, C. Noussair, and C. Plott. Nonspeculative bubbles in experimental asset markets: Lack of common knowledge of rationality vs. actual irrationality. *Econometrica*, 69(4):831–859, 2001. cited By 225.
- [80] Z.-Z. Li, R. Tao, C.-W. Su, and O.-R. Lobonç. Does bitcoin bubble burst? *Quality and Quantity*, 53(1):91–105, 2019. cited By 21.
- [81] T.-Y. Liu, H.-L. Chang, C.-W. Su, and X.-Z. Jiang. China’s housing bubble burst? *Economics of Transition*, 24(2):361–389, 2016. cited By 23.
- [82] R. Martin. The local geographies of the financial crisis: From the housing bubble to economic recession and beyond. *Journal of Economic Geography*, 11(4):587–618, 2011. cited By 237.
- [83] J. McDonald and H. Stokes. Monetary policy and the housing bubble. *Journal of Real Estate Finance and Economics*, 46(3):437–451, 2013. cited By 59.
- [84] J. Miao and P. Wang. Sectoral bubbles, misallocation, and endogenous growth. *Journal of Mathematical Economics*, 53:153–163, 2014. cited By 49.
- [85] J. Miao, P. Wang, and L. Xu. Stock market bubbles and unemployment. *Economic Theory*, 61(2):273–307, 2016. cited By 23.
- [86] J. Miao, P. Wang, and Z. Xu. A bayesian dynamic stochastic general equilibrium model of stock market bubbles and business cycles. *Quantitative Economics*, 6(3):599–635, 2015. cited By 30.
- [87] J. Michailova and U. Schmidt. Overconfidence and bubbles in experimental asset markets. *Journal of Behavioral Finance*, 17(3):280–292, 2016. cited By 22.
- [88] J. Miller and R. Ratti. Crude oil and stock markets: Stability, instability, and bubbles. *Energy Economics*, 31(4):559–568, 2009. cited By 341.

- [89] A. Nadler, P. Jiao, C. Johnson, V. Alexander, and P. Zak. The bull of wall street: Experimental analysis of testosterone and asset trading. *Management Science*, 64(9):4032–4051, 2018. cited By 17.
- [90] P. Narayan, S. Mishra, S. Sharma, and R. Liu. Determinants of stock price bubbles. *Economic Modelling*, 35:661–667, 2013. cited By 18.
- [91] S. Palan. A review of bubbles and crashes in experimental asset markets. *Journal of Economic Surveys*, 27(3):570–588, 2013. cited By 118.
- [92] A. Pavlov and S. Wachter. Robbing the bank: Non-recourse lending and asset prices. *Journal of Real Estate Finance and Economics*, 28(2-3):147–160, 2004. cited By 23.
- [93] D. Porter and V. Smith. Stock market bubbles in the laboratory. *Applied Mathematical Finance*, 1(2):111–128, 1994. cited By 55.
- [94] B. Roehner. Spatial analysis of real estate price bubbles: Paris, 1984-1993. *Regional Science and Urban Economics*, 29(1):73–88, 1999. cited By 32.
- [95] J. Rosser. Econophysics and economic complexity. *Advances in Complex Systems*, 11(5):745–760, 2008. cited By 32.
- [96] D. Sanders and S. Irwin. Bubbles, froth and facts: Another look at the masters hypothesis in commodity futures markets. *Journal of Agricultural Economics*, 68(2):345–365, 2017. cited By 19.
- [97] A. Scherbina and B. Schlusche. Asset price bubbles: A survey. *Quantitative Finance*, 14(4):589–604, 2014. cited By 37.
- [98] E. Schoenberg and E. Haruvy. Relative performance information in asset markets: An experimental approach. *Journal of Economic Psychology*, 33(6):1143–1155, 2012. cited By 18.
- [99] W. Semmler and B. Young. Lost in temptation of risk: Financial market liberalization, financial market meltdown and regulatory reforms. *Comparative European Politics*, 8(3):327–353, 2010. cited By 18.
- [100] W. Semmler and W. Zhang. Asset price volatility and monetary policy rules: A dynamic model and empirical evidence. *Economic Modelling*, 24(3):411–430, 2007. cited By 16.
- [101] S. Sharma and D. Escobari. Identifying price bubble periods in the energy sector. *Energy Economics*, 69:418–429, 2018. cited By 20.
- [102] S. Shi, J.-B. Jou, and D. Tripe. Can interest rates really control house prices? effectiveness and implications for macroprudential policy. *Journal of Banking and Finance*, 47(1):15–28, 2014. cited By 25.
- [103] Y.-N. Shih, H.-C. Li, and B. Qin. Housing price bubbles and inter-provincial spillover: Evidence from china. *Habitat International*, 43:142–151, 2014. cited By 41.
- [104] J. Siegel. What is an asset price bubble? an operational definition. *European Financial Management*, 9(1):11–24, 2003. cited By 47.
- [105] A. Smith, T. Lohrenz, J. King, P. Montague, and C. Camerer. Irrational exuberance and neural crash warning signals during endogenous experimental market bubbles. *Proceedings of the National Academy of Sciences of the United States of America*, 111(29):10503–10508, 2014. cited By 37.
- [106] V. Smith, M. Van Boening, and C. Wellford. Dividend timing and behavior in laboratory asset markets. *Economic Theory*, 16(3):567–583, 2000. cited By 55.



- [107] D. Sornette. Physics and financial economics (1776-2014): Puzzles, ising and agent-based models. *Reports on Progress in Physics*, 77(6), 2014. cited By 138.
- [108] D. Sornette and P. Cauwels. 1980–2008: The illusion of the perpetual money machine and what it bodes for the future. *Risks*, 2(2):103–131, 2014. cited By 32.
- [109] D. Sornette, R. Woodard, W. Yan, and W.-X. Zhou. Clarifications to questions and criticisms on the johansen-ledoit-sornette financial bubble model. *Physica A: Statistical Mechanics and its Applications*, 392(19):4417–4428, 2013. cited By 40.
- [110] K. Steiglitz and D. Shapiro. Simulating the madness of crowds: Price bubbles in an auction-mediated robot market. *Computational Economics*, 12(1):35–59, 1998. cited By 16.
- [111] C.-W. Su, K.-H. Wang, H.-L. Chang, and A. Dumitrescu-Peculea. Do iron ore price bubbles occur? *Resources Policy*, 53:340–346, 2017. cited By 19.
- [112] G. Svendsen. A general model for co2 regulation: The case of denmark. *Energy Policy*, 26(1):33–44, 1998. cited By 16.
- [113] M. Taylor and D. Peel. Periodically collapsing stock price bubbles: A robust test. *Economics Letters*, 61(2):221–228, 1998. cited By 55.
- [114] J. Ventura. Bubbles and capital flows. *Journal of Economic Theory*, 147(2):738–758, 2012. cited By 25.
- [115] S. Wadhvani. Should monetary policy respond to asset price bubbles? revisiting the debate. *National Institute Economic Review*, 206(1):25–34, 2008. cited By 24.
- [116] K. Watanabe, H. Takayasu, and M. Takayasu. A mathematical definition of the financial bubbles and crashes. *Physica A: Statistical Mechanics and its Applications*, 383(1 SPEC. ISS.):120–124, 2007. cited By 25.
- [117] W. Yan, R. Woodard, and D. Sornette. Diagnosis and prediction of tipping points in financial markets: Crashes and rebounds. volume 3, pages 1641–1657, 2010. cited By 32.
- [118] M. Yiu, J. Yu, and L. Jin. Detecting bubbles in hong kong residential property market. *Journal of Asian Economics*, 28:115–124, 2013. cited By 82.
- [119] M. Youssefmir, B. Huberman, and T. Hogg. Bubbles and market crashes. *Computational Economics*, 12(2):97–114, 1998. cited By 30.
- [120] D. Zhang, Z. Liu, G.-Z. Fan, and N. Horsewood. Price bubbles and policy interventions in the chinese housing market. *Journal of Housing and the Built Environment*, 32(1):133–155, 2017. cited By 22.
- [121] Q. Zhang, D. Sornette, M. Balcilar, R. Gupta, Z. Ozdemir, and H. Yetkiner. Lppls bubble indicators over two centuries of the s&p 500 index. *Physica A: Statistical Mechanics and its Applications*, 458:126–139, 2016. cited By 17.
- [122] Y.-J. Zhang and J. Wang. Exploring the wti crude oil price bubble process using the markov regime switching model. *Physica A: Statistical Mechanics and its Applications*, 421(1):377–387, 2015. cited By 37.
- [123] Y.-J. Zhang and T. Yao. Interpreting the movement of oil prices: Driven by fundamentals or bubbles? *Economic Modelling*, 55:226–240, 2016. cited By 57.
